# Supplementary material for: Scalable and Congestion-aware Routing for Autonomous Mobility-on-Demand via Frank-Wolfe Optimization
Source: arXiv:1903.03697 source file (2019-03-08)
Supplement: Supplementary file 1 [file supplementary.tex]

\section{Supplementary material (AMoD with loss as TAP)}
\subsection{AMoD with customer loss}
We introduce the constant $c_l$ which corresponds to the cost of not servicing one unit of user. For every class of users $m\in M$ we introduce the variable $\ell_m$ with the constraint 
\begin{align}\label{eq:loss:bound}
    0\leq \ell_m \leq \lambda_m,\quad \forall m\in M.
\end{align}
We then introduce the following constraint, which substitutes constraint~(\ref{eq:tap:flow}),
\begin{align}
    \sum_{j\in V_i^+}x_{ijm}-\sum_{j\in V_i^-}x_{jim}&=\lambda_{im}-\ell_m,\quad \forall i\in V. \label{eq:loss:flow}
\end{align}
We also introduce an alternative to constraint~(\ref{eq:amod:flow})
\begin{align}\label{eq:loss:rebalance}
    \sum_{j\in V_i^+}x_{ijr}-\sum_{j\in V_i^-}x_{jir}&=r_i^l,\quad \forall i\in V,
\end{align}
where \[r_i^l\eqq \sum_{m\in M}\left(\indicator\{d_m=i\}-\indicator\{o_m=i\}\right)\lambda_m.\] 

\begin{definition}
The \emph{AMoD with loss problem} (\amodl) consists of minimizing the expression $F(\hat{\bm{x}})+G(\bm{\ell})$,
where \[G(\bm{\ell})=c_l\cdot \sum_{m\in M}\ell_m,\]
subject to constraints~(\ref{eq:tap:positive}),(\ref{eq:amod:positive}),(\ref{eq:loss:bound}),(\ref{eq:loss:flow}),(\ref{eq:loss:rebalance}).
\end{definition}

\todo{Explain the motivation behind this section. E.g., to demonstrate the generality of the approach.}
Similarly to the previous section, we show that \amodl can be viewed as a special instance of \tap. However, in this section the transformation is slightly more involved and requires to modify the \frankwolfe algorithm. 

Recall that in addition to the rebalancing of user requests, which occurs in \amod, we also need to allow that some of the user requests will not be fulfilled. In particular, $\ell_m$ denotes the number of unfulfilled requests for $m\in M$. In that case, we need to send only $\ell_m$ rebalancers to $o_m$. To achieve this more complex logic we modify $G$ into a larger graph $G''$. Additionally, we couple the task of a car driving a passenger, and rebalacing to another origin node, and treat it as a single action of one vehicle. This way it is easier to determine whether losing a specific customer is worthwhile, as this cost encompasses both the cost of driving a customer, and then the cost rebalancing to the the origin of another. This will become clear shortly. 

\subsection{The construction}
Define 
\[O\eqq\bigcup_{m\in M}\{o_m\},\quad D\eqq \bigcup_{m\in M}\{d_m\}\] 
to be the sets of all origin and destination vertices, respectively. We introduce the graph $G''=(V'',E'')$ as follows:
\[V''=V\cup \{n,n'\}\cup\{i'|i\in D\},\]
\[E''=\{(n,n')\}\cup E_{\text{in}}\cup E_{\text{out}}\cup E_{\text{between}} \cup E_{\text{end}}, E_{\text{self}},\]
where 
\begin{align*}
    E_{\text{in}}&=\{(i,j)|(i,j)\in E, i\not\in D\},\\
    E_{\text{out}}&=\{(i',j)|(i,j)\in E, i\in D\},\\
    E_{\text{between}}&=\{(i,i')|i\in D\},\\
    E_{\text{end}}&=\{(i,n)|i\in D\},\\ 
    E_{\text{self}}&=\{(i',i)|i\in D, i\in O\}.\\
\end{align*}
\todo{Explain the purpose of $E_{\text{self}}$.}
We also assign costs $c'_{ij}$ for the edges in the following manner ($c_{ij}$ denotes the original cost with respect to $G$, if relevant):
for $(i,j)\in E_{\text{in}}\cup E_{\text{out}}$, $c'_{ij}(x_{ij})=c_{ij}(x_{ij})$ i.e., original cost; for $(i,j)\in E_{\text{between}}$, $c'_{ij}(x_{ij})=\eps\cdot x_{ij}$, where $\eps$ is a small constant (to be discussed below); for $(n,n')$, $c_{nn'}(x_{nn'})=c_l\cdot x_{nn'}$; 
for $(i,n)\in E_{\text{end}}$, $c'_{in}(x_{in})=\bpr(x_{in},\kappa_{in},L)$, where $L$ is defined as in the previous section and $\kappa_{in}=\sum_{m\in M}\indicator\{d_m=i\}$.

This requires some explanation. In addition to the dummy vertex $n$, which represents a destination for rebalancers that decided to fulfill passenger trips and rebalancing, we add the vertex $n'$ which would denote the destination for rebalancers that decided to stay idle. We add an additional copy $i'$ for every $i\in D$ (we assume that $i'$ is a new index that was not available in $V$). We add the edge $(n,n')$ as well as a slew of the following edges: Every edge $(i,j)\in E$ that does not terminate in a destination vertex in $G$ is added in $E_{\text{in}}$; every edge $(i,j)\in E$ that begins in a destination vertex is transformed into $(i',j)\in E_{\text{out}}$; an edge $(i,i')$ is drawn from $i\in D$ and its copy $i'$, in $E_{\text{between}}$, and $(i,n)$ is added from every destination vertex $i$, similarly to the previous section, in $E_{\text{end}}$. 

\subsection{Modified \allornothing assignment}
The purpose of this construction goes as follows: a car that begins its journey in $o_m$, for some $m\in M$ can be assigned with one of two actions: (i) it can remain \emph{idle}, in which case it will traverse the edges $(o_m,n),(n,n')$, or (ii) \emph{execute} the task, which includes traversing the shortest path from $o_m$ to $d'_m$, and then rebalancing by traversing the shortest path from $d'_m$ to $n$. This logic is described in the modified \allornothing assignment below (Algorithm~\ref{alg:aonl}), which is executed by \frankwolfe for the \amodl problem. 

To ensure that every destination vertex $i\in d$ receives the correct number of rebalancers, we assign to edge $(i,n)$ a capacity which is equal to the total arriving cars, idle or executing, similarly to the case of \amod.
We then extend the flow of idle cars to the edge $(i,n)$ and cost $c_l\cdot x_{nn'}$ to penalize idle cars. The final ingredient of duplicating destination vertices $i\in D$ into $i'$ guarantees that a request of computing a shortest path from a destination $i$ to $n$ will not use the edge $(i,n)$. Indeed, the execution task traverses a shortest path from $o_m$ to $d'_m$, where the latter vertex is not connected directly to $n$. \todo{Explain the purpose of $\eps$ edges.}

\begin{algorithm}\label{alg:aonl}
\caption{\allornothingloss$(G'',\nabla\bar{F}_E(\x^k),OD)$}
	\begin{algorithmic}[1]
		\For {$m\in M$}
		\State{$\y_m\gets \shortestpath(G'',\nabla\bar{F}_E(\x^k),o_m,d'_m)$}
		\State{$\y'_m\gets \shortestpath(G'',\nabla\bar{F}_E(\x^k),d'_m,n)$}
		\State{$\y^{\text{exe}}_m=\y_m+\y'_m$}
		\State{$c_{\text{exe}}=\nabla\bar{F}_E(\x^k)^T \y^{\text{exe}}_m$}
		\State{$\y^{\text{idle}}_m= \y(o_m,n)+\y(n,n')$}
		\State{$c_{\text{idle}}=\nabla\bar{F}_E(\x^k)^T \y^{\text{idle}}_m$}
		\If {$c_{\text{idle}}<c_{\text{exe}}$}
		\State{$\y^k_m =\y^{\text{idle}}_m$}
		\Else
		\State {$\y^k_m =\y^{\text{exe}}_m$}
		\EndIf
		\EndFor	
		\State 	\Return $\y^{k} = \sum_{m\in M}\lambda_m y^k_m$
	\end{algorithmic}
\end{algorithm}

We now review Algorithm~\ref{alg:aonl}. $\y_m,\y'_m$ represent the shortest paths from $o_m$ to $d'_m$, and from $d'_m$ to $n$, respectively (lines~2,3). The concatenation of the two paths is denoted by $\y^{\text{exe}}_m$ (line~4), where the cost of the entire execution is described by $c_{\text{exe}}$ (line 5). In line~6 we compute the $\y_m^\text{idle}$ which represent an idle rebalancer. The notation $\y(i,j)$ represents assigning $x_{ij}=1$, and $x_{i'j'}=0$ if $i'\neq i\vee j'\neq j$. Its cost is denoted by $c_\text{idle}$ (line~7). The minimal-cost action is chosen in lines~8-11. 

Observe that this modified \allornothing routine ensures that for every request $m$ the total number of cars executing or idling over request $(o_m,d_m)$ is exactly $\lambda_i$. Furthermore, this property is maintained from one iteration of \frankwolfe to the next, due to the averaging performed in line~5 of Algorithm~\ref{alg:fw}.
